# Supplementary material for: Creativity: Generating Diverse Questions using Variational Autoencoders
Source: arXiv:1704.03493 source file (2017-04-11)
Supplement: Supplementary file 1 [file supp.tex]

%\section{Supplementary Material}

\begin{table}[h]
\centering
\begin{tabular}{l c c c c c c}
\hline
Sampling & Avg. Bleu & Oracle Bleu & Avg. Meteor  & Oracle Meteor & UQ & Unseen UQ \\ \hline
N1, 100 & \textbf{0.331} & 0.37 & \textbf{0.188 } & 0.207 & 1.78  & 6.54 \\
N1, 500  &  0.328 &0.376       &0.187   &0.211     &2.04     &7.44 \\
U10, 100 &0.305 & 0.447&0.178 & 0.254& 2.04& 7.44\\
U10, 500 & 0.295&0.468 &0.175 & 0.269&12.52 & 16.22\\
U20, 100 & 0.295& 0.486& 0.172 &0.281& 17.02& 13.66\\
U20, 500 & 0.283& \textbf{0.519}& 0.168& \textbf{0.307}& \textbf{33.41}& \textbf{19.6}\\
\hline
\end{tabular}
\centering
\caption{VQG-COCO Summary of metrics. Metrics \textbf{averaged} over the epochs.}
\label{tab:metrics_coco_avg}
\end{table}

\begin{table}[h]
\centering
\begin{tabular}{l c c c c c c}
\hline
Sampling & Avg. Bleu & Oracle Bleu & Avg. Meteor  & Oracle Meteor & UQ & Unseen UQ \\ \hline
N1, 100 	&	\textbf{0.305 }	& 	0.346 	&	\textbf{0.165}	& 0.181 & 1.88  &	9.64\\
N1, 500  	&  	0.302 	&	0.351	&	\textbf{0.165 }  & 0.185 & 2.18  &	10.87\\
U10, 100 	&	0.283 	& 	0.417	&	0.160	& 0.221 & 9.07  &	16.31\\
U10, 500 	& 	0.275	&	0.436	&	0.158	& 0.234 & 14.73 &	20.59\\
U20, 100 	& 	0.278	& 	0.453	&	0.157	& 0.245 & 18.93 &	16.66\\
U20, 500	& 	0.267	& 	\textbf{0.483}	&	0.154	& \textbf{0.267} & \textbf{39.01} &	\textbf{22.6}\\
\hline
\end{tabular}
\centering
\caption{VQG-Flickr Summary of metrics. Metrics \textbf{averaged} over the epochs.}
\label{tab:metrics_flickr_avg}
\end{table}

\begin{table}[h]
\centering
\begin{tabular}{l c c c c c c}
\hline
Sampling & Avg. Bleu & Oracle Bleu & Avg. Meteor  & Oracle Meteor & UQ & Unseen UQ \\ \hline
N1, 100 	&	\textbf{0.295} 	& 	0.336 	&	\textbf{0.165}	& 0.183 & 1.98  &	15.56\\
N1, 500  	&  	0.292 	&	0.342	&	0.164   & 0.187 & 2.31  &	17.00\\
U10, 100 	&	0.277 	& 	0.415	&	0.159	& 0.228 & 10.17  &	23.43\\
U10, 500 	& 	0.267	&	0.436	&	0.157	& 0.242 & 16.94 &	28.83\\
U20, 100 	& 	0.272	& 	0.452	&	0.155	& 0.252 & 21.06 &	23.65\\
U20, 500	& 	0.261	& 	\textbf{0.482}	&	0.152	& \textbf{0.273} & \textbf{44.65} &	\textbf{30.73}\\
\hline
\end{tabular}
\centering
\caption{VQG-Bing Summary of metrics. Metrics \textbf{averaged} over the epochs.}
\label{tab:metrics_bing_avg}
\end{table}

% Max over epochs:

\begin{table}[h]
\centering
\begin{tabular}{l c c c c c c}
\hline
Sampling & Avg. Bleu & Oracle Bleu & Avg. Meteor  & Oracle Meteor & UQ & Unseen UQ \\ \hline
N1, 100 & \textbf{0.356} & 0.393 & \textbf{0.199 } & 0.219 & 1.98  & 10.76 \\
N1, 500  &  0.352 &0.401       &0.198   &0.222     &2.32     &12.19 \\
U10, 100 &0.328 & 0.488&0.19 & 0.275& 9.82& 18.78\\
U10, 500 & 0.326&0.511 &0.186 & 0.291&16.14& 24.32\\
U20, 100 & 0.316& 0.544& 0.183 &0.312& 22.01& 19.75\\
U20, 500 & 0.311& \textbf{0.579}& 0.177& \textbf{0.342}& \textbf{46.1}& \textbf{27.88}\\
\hline
\end{tabular}
\centering
\caption{VQG-COCO Summary of metrics. These metric values are the \textbf{maximum} over the epochs.}
\label{tab:metrics_coco_max}
\end{table}

\begin{table}
\centering
\begin{tabular}{l c c c c c c}
\hline
Sampling & Avg. Bleu & Oracle Bleu & Avg. Meteor  & Oracle Meteor & UQ & Unseen UQ \\ \hline
N1, 100 	&	\textbf{0.335 }	& 	0.365 	&	\textbf{0.176}	& 0.191 & 2.17  &	15.2\\
N1, 500  	&  	0.333 	&	0.374	&	0.174   & 0.193 & 2.63  &	17.1\\
U10, 100 	&	0.314 	& 	0.456	&	0.168	& 0.241 &12.21 &	25.65\\
U10, 500 	& 	0.31	&	0.479	&	0.167	& 0.254 & 21.14 &	32.12\\
U20, 100 	& 	0.304	& 	0.509	&	0.166	& 0.276 & 26.83 &	24.98\\
U20, 500	& 	0.299	& 	\textbf{0.541}	&	0.163	& \textbf{0.3} & \textbf{59.57} &	\textbf{33.81}\\
\hline
\end{tabular}
\centering
\caption{VQG-Flickr Summary of metrics. These metric values are the \textbf{maximum} over the epochs.}
\label{tab:metrics_flickr_max}
\end{table}

\begin{table}
\centering
\begin{tabular}{l c c c c c c}
\hline
Sampling & Avg. Bleu & Oracle Bleu & Avg. Meteor  & Oracle Meteor & UQ & Unseen UQ \\ \hline
N1, 100 	&	\textbf{0.316} 	& 	0.357 	&	\textbf{0.175}	& 0.194 & 2.32  &	22.15\\
N1, 500  	&  	0.315 	&	0.364	&	0.173   & 0.198 & 2.76  &	22.87\\
U10, 100 	&	0.304 	& 	0.457	&	0.168	& 0.252 & 12.99  &	32.84\\
U10, 500 	& 	0.299	&	0.481	&	0.166	& 0.266 & 23.3 &	39.84\\
U20, 100 	& 	0.296	& 	0.503	&	0.164	& 0.286 & 27.71 &	32.91\\
U20, 500	& 	0.291	& 	\textbf{0.538}	&	0.161	& \textbf{0.311} & \textbf{63.83} &	\textbf{42.58}\\
\hline
\end{tabular}
\centering
\caption{VQG-Bing Summary of metrics. These metric values are the \textbf{maximum} over the epochs.}
\label{tab:metrics_bing_max}
\end{table}
